# Supplementary material for: Toward Cloud Tomography from Space using MISR and MODIS: The Physics of Image Formation for Opaque Convective Clouds
Source: arXiv:2011.14537 ancillary file (2021-07-27)
Supplement: Supplementary file 1 [file paper_veiled_core_physics-eSupA.pdf]

## APPENDIX A

**Angular smearing: The directionally-correlated random walk approach****1) RADIATIVE TRANSFER (RT) AS A RANDOM WALK WITH DIRECTIONAL CORRELATION**

We wish to compute some statistical properties of particles in a directionally-correlated random walk (RW) in a uniform unbounded 3D space in order to investigate Green functions or point spread functions (PSFs) of scattering optical media such as clouds. These RWs depart from the origin ( $x = y = z = 0$ ) in direction  $\Omega_0 = \hat{\mathbf{z}}$ , the unit vector along the  $z$ -axis. After  $N$  steps (i.e., propagations and scatterings), we have a random cumulative position

$$\mathbf{x}_N = \sum_{n=0}^{N-1} s_{n+1} \Omega_n \quad (\text{A1})$$

where  $s_n$  is the  $n^{\text{th}}$  random step magnitude and  $\Omega_n$  the  $n^{\text{th}}$  direction of propagation, with the convention that  $\mathbf{x}_0 = \mathbf{0}$ . We know that  $\Omega_n$  and  $\Omega_{n+1}$  are correlated in the sense that the random scattering angle  $\theta_s = \cos^{-1} \Omega_n \cdot \Omega_{n+1}$  samples the forward-peaked phase function (PF)  $p(\theta_s)$ ,  $n \geq 0$ , viewed as an azimuthally-invariant 2D probability density function (PDF). By rotational symmetry around  $\hat{\mathbf{z}}$ , we know that  $\langle x_N \rangle = \langle \hat{\mathbf{x}} \cdot \mathbf{x}_N \rangle$  and  $\langle y_N \rangle = \langle \hat{\mathbf{y}} \cdot \mathbf{x}_N \rangle$  vanish. We then ask:

1. What is the ensemble average  $\langle z_N \rangle = \langle \hat{\mathbf{z}} \cdot \mathbf{x}_N \rangle$  over all possible trajectories?
2. What is the asymptotic limit of  $\langle z_N \rangle$  as  $N \rightarrow \infty$ ?
3. How fast is the convergence to the asymptotic limit?

We first note that  $s_n$  and  $\Omega_n$  are independent random variables, and that  $\mathbf{x}_N$  is in an optically uniform unbounded space. Thus, we have  $\langle \mathbf{x}_N \rangle = \ell \langle \mathbf{S}_N \rangle$ , where  $\ell = \langle s_n \rangle$ , for all  $n$ , is the particle mean-free-path (MFP). We have also defined  $\mathbf{S}_N = \sum_{n=0}^{N-1} \Omega_n$  as the sum of  $N$  random unit vectors correlated one-to-the-previous according to  $p(\Omega_n \cdot \Omega_{n+1})$  for  $n \geq 1$ , with the convention that  $\mathbf{S}_0 = \mathbf{0}$ . We thus wish to compute  $\langle z_N \rangle = \ell \langle M_N \rangle$ , where  $\langle M_N \rangle = \hat{\mathbf{z}} \cdot \langle \mathbf{S}_N \rangle$  is the component of  $\langle \mathbf{S}_N \rangle$  along the  $z$ -axis. By definition,  $\langle M_N \rangle = \sum_{n=0}^{N-1} \langle \mu_n \rangle$  where  $\mu_n$  is the  $z$ -component of  $\Omega_n$ , and  $\langle M_0 \rangle = 0$ .

Before any scattering, we have  $\langle \mu_0 \rangle = 1$ . We also have  $\langle \mu_1 \rangle = g$  after a single scattering based on the definition of the asymmetry factor  $g$ , as the mean value of  $\mu_1 = \Omega_1 \cdot \hat{\mathbf{z}}$  averaged over the PF. In fact, we have

$$\langle \mu_n \rangle = \langle \Omega_n \cdot \hat{\mathbf{z}} \rangle = g^n. \quad (\text{A2})$$

Indeed, the sequence of step magnitudes  $s_n$  is just a randomly-ordered collection of random variables drawn

from the same probability distribution. Therefore, the sequence  $\{\Omega_n, n \geq 0\}$  is a RW on the unit sphere, generated by

$$\Omega(\mu_n, \phi_n) = \Omega(\mu_{n-1}, \phi_{n-1}) + \delta_n(\mu_s, \phi_s), \quad n \geq 1, \quad (\text{A3})$$

where  $\mu_s$  is drawn from the generally forward-peaked PF, and the scattering azimuth angle  $\phi_s$  is a uniform random variable on  $(-\pi, +\pi]$ . We have thus reduced the essence of the directionally-correlated RW  $\{\mathbf{x}_N, N \geq 0\}$  that is unfolding in an *infinite* Euclidian 3D space to a standard RW (i.e., uncorrelated steps)  $\{\Omega_N, N \geq 0\}$  on the unit sphere that, importantly here, is a *finite* curved 2D space. The directional equivalent of the MFP  $\ell = \langle s \rangle$  in 3D space is the mean angular magnitude of  $\delta_n(\mu_s, \phi_s)$  in (A3), namely, the polar angle

$$\theta_\delta = \cos^{-1} \langle \mu_s \rangle = \cos^{-1} g. \quad (\text{A4})$$

For typical cloud PFs, we have  $g \approx 0.85$  (liquid) or  $g \approx 0.75$  (ice), hence  $\theta_\delta \approx 31.8^\circ$  (liquid) and  $\theta_\delta \approx 41.4^\circ$  (ice). These are quite large steps across the spherical manifold, and we can anticipate that it will not take many steps for a large ensemble of RWs leaving the North pole to diffuse across the whole available space.

From spherical trigonometry, the random incrementation in (A3) is computed as

$$\mu_n = \mu_{n-1} \mu_s + \sqrt{1 - \mu_{n-1}^2} \sqrt{1 - \mu_s^2} \cos \phi_s,$$

and there are related expressions for the other two cartesian components of  $\Omega(\mu_n, \phi_n)$ . By averaging over the random increments  $\delta_n(\mu_s, \phi_s)$ , the second term vanishes due to the azimuthal symmetry of the PF, and we are left with

$$\langle \mu_n \rangle = \langle \mu_{n-1} \rangle \langle \mu_s \rangle = \langle \mu_{n-1} \rangle g,$$

hence (A2), by induction. From there,

$$\langle M_N \rangle = \sum_{n=0}^{N-1} g^n = \frac{1 - g^N}{1 - g}.$$

This leads immediately to the answer to our first question:

$$\langle z_N \rangle = \ell \langle M_N \rangle = \ell \frac{1 - g^N}{1 - g}, \quad (\text{A5})$$

which is numerically verified in Fig. A2a. The answer to our second question is therefore:

$$\ell_t = \lim_{N \rightarrow \infty} \langle z_N \rangle = \frac{\ell}{1 - g}, \quad (\text{A6})$$

which was defined in the main text as the “transport” or “scaled” MFP in the absence of absorption (single scattering albedo  $\omega = 1$ ). Transport MFP  $\ell_t$  was then used to quantify angular smearing via multiple scattering when

the PF is forward-peaked. Figure A1 illustrates the loss of directional memory in angularly-correlated RWs in unbounded 2D space as a consequence of the associated diffusion process in direction space.

The above computation of  $\langle z_N \rangle$  is easily generalized to the case of  $\omega < 1$  where there is a finite probability  $1 - \omega$  of terminating the RW at every step because the particle is absorbed at the point of scattering. After  $n$  scatterings, the probability of surviving this iterated Bernoulli trial is  $\omega^n$ . Therefore,  $\langle z_N \rangle = \ell \sum_{n=0}^{N-1} (\omega g)^n$ , and  $\ell_t = \langle z_\infty \rangle$  becomes identical to Eq. (13) in the main text.

As anticipated, and in sharp contrast with the RW  $\mathbf{S}_N$  ( $N \geq 0$ ) in 3D space, the RW  $\Omega_n$  ( $n \geq 0$ ) on the sphere—a finite space—quickly covers all of it. To estimate how fast, we ask how many steps until the average  $z$ -axis component  $\langle \mu_n \rangle$  in (A2) becomes  $\ll 1$ . The answer is obtained by expressing the geometric series increment as  $g^n = e^{n \ln g} = e^{-n \ln(1/g)} \approx e^{-n(1/g-1)}$  in the limit  $g \rightarrow 1$ . This highlights the exponentially-decaying (a.k.a. “short-term”) directional memory, with a characteristic e-folding time  $\ln(1/g)^{-1} \approx (1/g - 1)^{-1} = g/(1 - g)$ . Another way of seeing this is to write (A5) as  $\langle z_N \rangle = \ell_t (1 - g^N)$  when  $N \gg 1$ , hence an exponential convergence rate in an e-folding time  $\ln(1/g)^{-1}$ . Note that, as expected on physical grounds, convergence of  $\langle z_N \rangle$  to  $\ell_t$  is achieved—and directional memory is lost—instantaneously (i.e., at  $N = 1$ ) when  $g = 0$ .

That answers our third and last important question about how many scatterings it takes to forget what the original direction of propagation is:

$$n_{\text{smear}} = \frac{1}{\ln(1/g)} \approx \frac{1}{1/g - 1} = \frac{g}{1 - g} \quad (\text{A7})$$

if  $g \lesssim 1$ . To illustrate, we take the canonical  $g = 0.85$  (0.75) for liquid (ice) clouds, hence  $1/\ln(1/g) \approx 6.15$  (3.48). Alternatively, we have  $1 - g = 0.15$ , hence  $g/(1 - g) \approx 5.76$  (3.00). In short,  $n = 5$  or  $6$  ( $\approx 3$ ) scatterings gets  $\langle \mu_n \rangle$  to  $1/e \approx 0.37$ , and doubling that number to 10 to 12 ( $\approx 6$ ) scatterings reduces  $\langle \mu_n \rangle$  to  $1/e^2 \approx 0.13$ . At those milestones, the indicator polar angle  $\cos^{-1} \langle \mu_n \rangle$  is  $68^\circ$  ( $82^\circ$ ), which can be interpreted as how far the propagation direction has drifted away from  $0^\circ$ .

## 2) FROM DIRECTIONAL TO SPATIAL DIFFUSION

Knowing that the MFP for the RW  $\{\Omega_n, n \geq 0\}$  on the unit sphere is  $\theta_g$  in (A4), we ask about the whole distribution of random isotropic (i.e., azimuthally symmetric) steps. For  $n = 1$ , it is of course just the azimuthally-symmetric scattering PF. That makes it the spherical counterpart of the exponential distribution of step sizes,  $s$ , from Beer’s law of direct transmission in uniform media that, in

turn, generates the RW  $\{\mathbf{x}_n, n \geq 0\}$  in 3D space. A well-known instance (used, e.g., in Fig. A1) is the Henyey–Greenstein (HG) PF (Henyey and Greenstein 1941)

$$p_g(\mu_s) = \left( \frac{1}{4\pi} \right) \frac{1 - g^2}{(1 + g^2 - 2g\mu_s)^{3/2}}, \quad (\text{A8})$$

which is uniquely determined by its asymmetry factor  $\langle \mu_s \rangle = g$ . A corollary of the result in (A2) is that the class of HG PFs is closed under the angular convolution product. Indeed, any sum of random variables, as in (A3), implies a convolution of their PDFs. On the sphere, the convolution of two functions is done by multiplying term-by-term their Legendre coefficients.<sup>1</sup> Legendre expansion coefficients of a HG PF  $p_g(\mu_s)$  are  $(2m + 1)g^m$  ( $m \geq 0$ ). Legendre expansion coefficients of a HG PF convolved with itself are therefore  $(2m + 1)(g^2)^m$  ( $m \geq 0$ ), which is a HG PF with parameter  $g_2 = g^2$ . After  $n$  steps, the PDF of the angular distribution is still HG function, now with  $g_n = g^n$ . As estimated in the above, it is rapidly approaching  $g_\infty = 0$ , i.e., an isotropic PDF on the sphere.

For the RW  $\{\mathbf{x}_n, n \geq 0\}$  in unbounded 3D space, as defined by (A1), there is also an iterated convolution product at work. The PDF for every one of the random steps  $s$  is an exponential distribution with mean  $\ell$ , which is also the standard deviation. Moreover, we showed in the above that after a finite number of steps,  $\sim 10$  to  $12$ , directional memory is all but lost in liquid clouds where  $g \approx 0.85$ . Consequently, the spatial distribution of randomly walking particles, irrespective of direction, results from the convolution of  $\sim 10$  to  $12$  random steps with rapidly decaying angular correlation. Under these conditions, we can safely surmise that, since step variance  $\ell^2$  is finite, the PDF of the the sum total  $\mathbf{x}_n$  for  $n \approx 11$  is close-to-gaussian, by virtue of the central limit theorem, in all three directions. Along the  $z$ -axis, the mean is computed analytically in (A5) while along the  $x$ - and  $y$ -axes the means vanish by rotational symmetry of the scattering PF. As shown numerically in Fig. A1, the dispersion (measured by the standard deviation) in  $z$  increases with  $n$ , and the same happens for  $x$ , and for  $y$  too in 3D space.<sup>2</sup> Just as the isotropic PDF in direction space is the attractor for repeated angular convolutions of PFs with any width, the gaussian PDF is the attractor for any step distribution with finite variance.<sup>3</sup>

<sup>1</sup>This is the spherical counterpart of the conversion of convolution products of functions in Euclidian spaces to standard products of their Fourier transforms, a.k.a. “characteristic functions” in probability theory. On the 2D sphere, the counterpart of the Fourier expansion is indeed the spherical harmonics expansion.

<sup>2</sup>Further additions of normally distributed random variables only lead to wider quasi-gaussian PDFs.

<sup>3</sup>For step distributions with divergent variance, the attractors are Lévy-stable PDFs. See Davis and Marshak (1997) for ramifications in 1D RT through *homogenized* plane-parallel media where the free-path distribution accounts statistically for the spatial variability expected in turbulent optical media such as cloudy atmospheres.

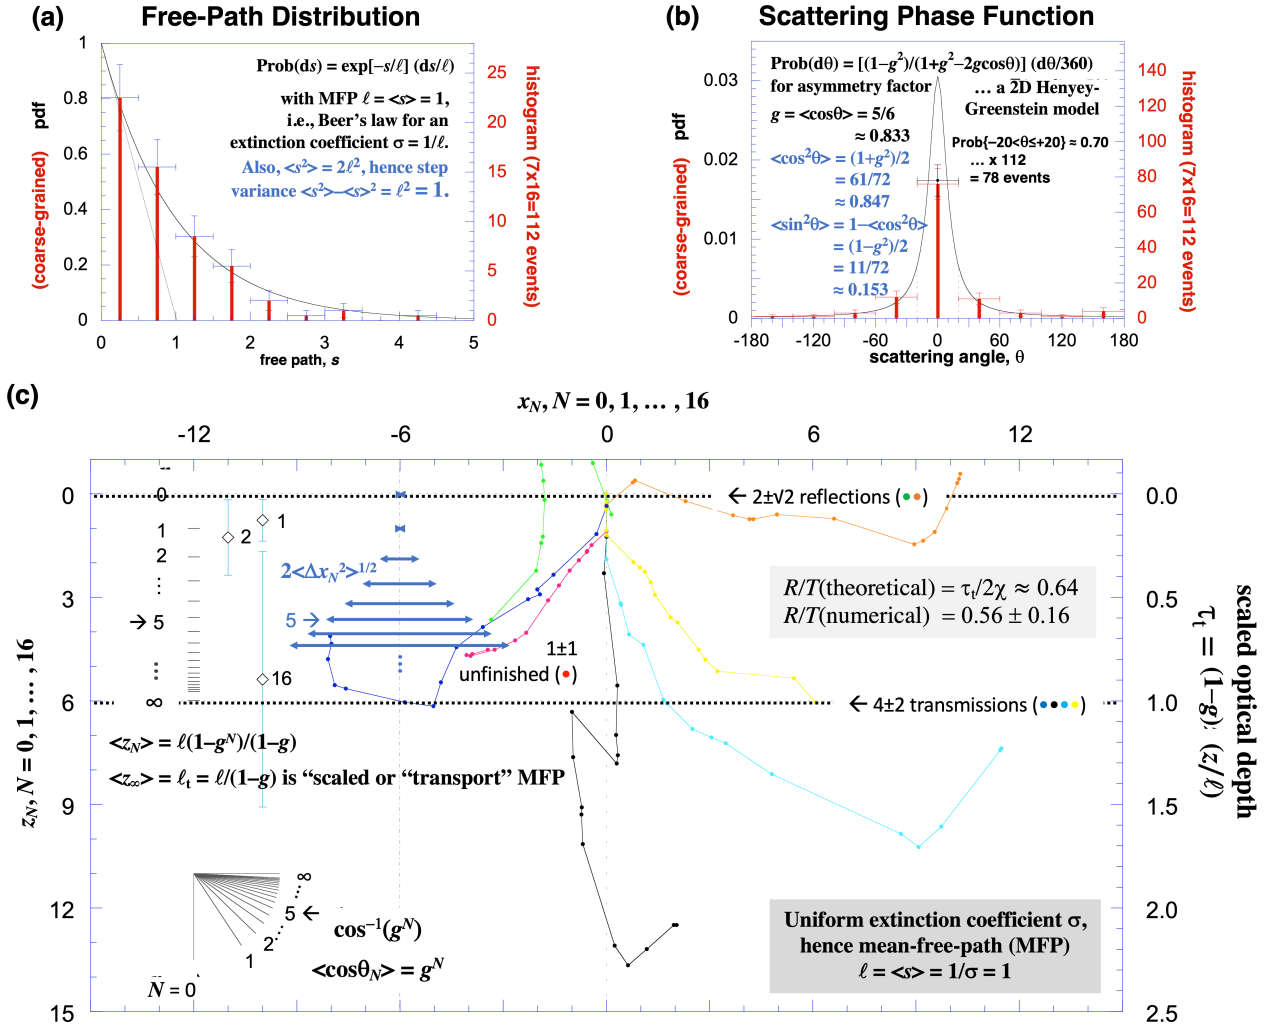

FIG. A1. Rescaling of the MFP due to forward-peaked scattering in a uniform 2D medium and associated lateral transport. **(a)** Beer's exponential law of extinction that dictates the distribution of free paths  $s$ :  $\Pr\{\text{step} \geq s\} = \exp(-s/\ell)$  with unit mean ( $\ell = \langle s \rangle = 1$ ). **(b)** The scattering kernel  $p(\theta_s)$  is the 2D counterpart of the HG model in (A8) is used; this PDF describes the distribution of scattering angle  $\theta_s$ , with an asymmetry factor  $g = \langle \cos\theta_s \rangle = 5/6 \approx 0.83$ . In panels (a-b), error bars are based on the expected means and (Poissonian) variances, given the number of events per bin for a total of  $7 \times 16 = 112$  samples. **(c)** Seven 2D directionally-correlated RWs, all starting straight down at the origin, all 16 steps long. The left-hand scale is in MFPs; the right-hand  $z$ -axis uses transport MFPs from Eq. (A6). In the lower l.-h. corner, an indication of the average direction of travel is plotted for  $N = 0, 1, \dots, 16$  and  $\infty$ ; in the upper l.-h. corner, the corresponding theoretical average positions are indicated for orders-of-scattering  $N = 0, 1, \dots, 16$  and  $\infty$ , and again for  $N = 1, 2, 16$  but obtained empirically (with standard deviations). After a number of anisotropic scatterings, a particle in a directionally-correlated RW may just as well have been scattered just once but isotropically, with the MFP for such a scattering being longer by a factor  $1/(1-g) = 6$ . The characteristic  $n_{\text{smear}} \approx (1/g - 1)^{-1} = 5$  from (A7) is highlighted. To the left of the trajectories, horizontal blue-hued double arrows centered at  $(-6, \langle z_N \rangle)$  indicate twice the standard deviation of  $x_N$ , that is,  $2\langle x_N^2 \rangle^{1/2}$  ( $N = 0, 1, \dots, 7$ ), as computed numerically for the 2D HG PF with  $g = 5/6$ . Although there are only 7 trajectories, tallies for  $R$  and  $T$  are performed for a vertically finite plane-parallel medium with optical thickness  $\tau = z/\ell = 1/(1-g) = 6$ , i.e., upper and lower boundaries at 0 and  $\tau_1 = 1$ , respectively. The outcome for  $R/T$  is compared with the theoretical prediction from Davis (2002), using  $\chi = \pi/4$  for the diffusion limit in 2D RT. Adapted from Fig. 7 in Davis and Marshak (1997).

That is key to the transition from discrete-time RW formalism used here to the continuous-time formulation that is implicit in the radiative diffusion model used in App. B. Gaussians with variance increasing linearly in time are the fundamental solution to the archetype of parabolic PDEs:

$\partial_{ct} J = D \nabla^2 J$  where  $J(ct, \mathbf{x})$  is the ensemble average density of WRing particles with path length  $ct$  at point  $\mathbf{x}$ . Diffusivity  $D = \ell_1/3$  in 3D space, and the Green function initial condition is  $J(ct, \mathbf{x})|_{ct=0} = \delta(\mathbf{x})$ . The diffusive radiation transport equation adopted in App. B is simply the

elliptical Laplace PDE for steady-state radiative diffusion, namely,  $\nabla^2 J = 0$ , with boundary conditions that express the distribution of boundary sources.

### 3) FROM LONGITUDINAL DRIFT TO LATERAL DISPERSION, AND BACK

The gradual movement of the mean value of  $z_N$  as  $N$  increases in (A5) is, in essence, a systematic drift along the original direction of propagation, ending when directional memory is all but lost, i.e., when  $N$  exceeds  $n_{\text{smear}}$  in (A7) and  $\langle z_N \rangle$  approaches the transport MFP (A6). The multiple scattering also causes a lateral dispersion of the narrow collimated light beam, sometimes called “blooming.” This horizontal spread also needs to be quantified here since, by reciprocity, it defines the size of the blurred image of a point source of light at a depth of  $\langle z_N \rangle$  into the scattering medium captured by a remote overhead sensor. This requires consideration of the increasing variances of the RW coordinates  $(x_N, z_N)$  as functions of  $N \geq 0$ .

Figure A1 shows numerically-computed standard deviation of  $x_N$  drawn to scale as blue double-headed arrows of length  $2\langle x_N^2 \rangle^{1/2}$  for the 2D HG PF with  $g = 5/6 \approx 0.83$ . Analytically, one needs to compute  $\langle (\sum_{n=0}^{N-1} s_{n+1} \sin \theta_n)^2 \rangle$  where the  $N$  random steps  $s_{n+1}$  and directions  $\theta_n$  are independent of each other at any given step. The lengths  $s_{n+1}$  of the  $N$  steps are all independent. The directions  $\theta_n$  however are not since there are angular correlations to the next and previous ones in the sequence due to the forward-peaked scattering. Noting that  $\langle x_N \rangle$  vanishes due to rotational symmetry of the PF and choice of original direction (along  $z$ -axis), variance of  $x_N$  is

$$\begin{aligned} \langle x_N^2 \rangle &= \left\langle \left( \sum_{n=0}^{N-1} s_{n+1} \sin \theta_n \right)^2 \right\rangle \\ &= \sum_{n=0}^{N-1} \langle s_{n+1}^2 \rangle \langle \sin^2 \theta_n \rangle \\ &\quad + 2 \sum_{n>m} \langle s_{n+1} \rangle \langle s_{m+1} \rangle \langle \sin \theta_n \sin \theta_m \rangle \\ &= 2\ell^2 \left[ \sum_{n=0}^{N-1} \langle \sin^2 \theta_n \rangle \right. \\ &\quad \left. + \sum_{n>m} \langle \sin \theta_n \sin \theta_m \rangle \right], \end{aligned} \quad (\text{A9})$$

where we used the independencies and that, for exponentially distributed steps,  $\langle s^2 \rangle = 2\ell^2$ . We see right away that  $\langle x_0^2 \rangle = \langle x_1^2 \rangle = 0$ , firstly by convention for  $x_0$  and secondly because we start with  $\theta_0 = 0$ .

Now, for 2D RWs,  $\theta_n = \sum_{i=1}^n \theta_{si}$ , the sum of all scattering angles, which are independent, from first to last, assuming  $\theta_0 = 0$ . Thus,  $\sin \theta_n = 2 \sin \theta_{sn} \cos \theta_{n-1}$ , where  $\theta_{sn}$  and  $\theta_{n-1}$  are independent. Therefore,

$\langle \sin \theta_n \rangle = 2 \langle \sin \theta_{sn} \rangle \langle \cos \theta_{n-1} \rangle = 0$ , because the first term vanishes per PF symmetry. However,  $\langle \sin^2 \theta_n \rangle = 4 \langle \sin^2 \theta_{sn} \rangle \langle \cos^2 \theta_{n-1} \rangle = 4(1 - \langle \cos^2 \theta_{sn} \rangle) \langle \cos^2 \theta_{n-1} \rangle$  does not vanish, and can be computed recursively. Indeed, for the 2D HG PF expressed in Fig. A1 and using previous notation for the cosines, we have  $\langle \mu_s^2 \rangle = (1 + g^2)/2$ , hence  $\langle \sin^2 \theta_{sn} \rangle = 1 - \langle \mu_s^2 \rangle = (1 - g^2)/2$ , for any  $n$ . In the above, we showed that  $\langle \mu_{n-1} \rangle = g^{n-1}$ , for  $n > 0$  and, by convention,  $\mu_0 = 0$ . We also noted previously that the running sum of step directions is tantamount to iterative convolutions of the PF with itself, and that self-convolved HG PFs are still HG PFs with the asymmetry parameter  $g$  squared. Therefore,  $\langle \mu_{n-1}^2 \rangle = (1 + g^{2(n-1)})/2$  for  $n \geq 1$ .

In summary, we have all the information we need to compute the summand in the first sum in (A9), namely,  $\langle \sin^2 \theta_n \rangle = (1 - g^2)(1 + g^{2(n-1)})$  for  $n \geq 1$ . The first term in (A9) is a lower bound on the variance of  $x_N$ , where global directional correlations along each RW in the second term, a double summation, are neglected. Thus,

$$\begin{aligned} \langle x_N^2 \rangle / \ell^2 &\geq 2 \sum_{n=0}^{N-1} \langle \sin^2 \theta_n \rangle \\ &= 2 \sum_{n=1}^{N-1} (1 - g^2)(1 + g^{2(n-1)}) \quad (\text{A10}) \\ &= 2 \left( (1 - g^2)(N - 1) + 1 - g^{2(N-1)} \right), \end{aligned}$$

for  $N \geq 1$ , by identifying the constant-term and geometric truncated series. Equality applies for  $N = 1, 2$  (in the later case because  $\sin \theta_0 = 0$  cancels the second term in (A9)), and the inequality holds for larger numbers of steps. Recall that, by convention,  $\langle x_0^2 \rangle = 0$ .

We anticipate a gradual increase in variance for  $x_N$  above the estimate in (A10). The magnitude of the correlation terms in the double summation in (A9) will necessarily decrease as  $(n, m)$  moves away from the diagonal. Assuming for simplicity that they vanish for  $n - m$  above some finite value, which is consistent with the short (exponentially-decaying) nature of directional memory, the magnitude of the double sum increases linearly with  $N$ . Figure A2c compares theoretical and numerical estimates of the standard deviation  $\langle x_N^2 \rangle^{1/2} / \ell$  for unbounded space (black curves). As expected, the former is a lower bound for the later, and the total variance is quickly dominated by the cross-correlation contribution. That said, Fig. A2c shows that numerical estimates of  $\langle x_N^2 \rangle^{1/2} / \ell$  for  $N \lesssim 10$  follow a near-linear proportionality in  $N - 1$ . Since the analytical model is exact for  $N = 1, 2$ , we have a closed-form prediction for the slope of this linear function, namely, the  $N = 2$  value from (A10):  $4(1 - g^2)$  for the 2D HG PF. This suggests a semi-analytical expression for  $\langle x_N^2 \rangle^{1/2} / \ell = \max\{0, 2\sqrt{1 - g^2}(N - 1)\}$  for  $0 \leq N \lesssim 10$ , at least when  $g \approx 5/6$ . The upper bound in  $N$  may depend on  $g$  and on dimensionality, but will likely always cover the radiative boundary layer.

For large enough  $N$ , the RW enters an asymptotic regime where variance in all coordinates increases linearly with  $N$  at a rate that is proportional to the transport MFP in (A6) squared and inversely proportional to  $n_{\text{smear}}$  in (A7), as indicated in Fig. A2c for  $x_N$  and in Fig. A2b for  $z_N$  (unbounded case only).

We now return to the vertical coordinate  $z_N$  of the directionally-correlated RW. In previous sections, we computed the ensemble mean  $\langle z_N \rangle$  in (A5) for RW in *unbounded* 1D, 2D or 3D spaces. That theory is exact because means of each step projected onto the  $z$ -axis are additive, whether or not they are statistically correlated. As we are reminded in the above with  $x_N$ , that is no longer true for variances: covariances in (A9) matter, and neglecting them in (A10) only yields a rather weak lower bound.

We can write a definition for the 2nd-order moment of  $z_N$  simply by changing the sines to cosines in (A9). Then, to get its variance, we subtract  $\langle z_N \rangle^2$ . Since we will again forego the increasingly many cross-correlation terms,  $\langle \cos \theta_n \cos \theta_m \rangle$ , as  $N$  increases, we will get a lower bound for the variance of  $z_N$  by summing the variances for all the increments  $s_{n+1} \cos \theta_n$  ( $n \geq 0$ ), where the step and cosine are independent. Thus,  $\langle s_{n+1}^2 \cos^2 \theta_n \rangle = 2\ell^2 \langle \cos^2 \theta_n \rangle$ . For the 2D HG PF,  $\langle \cos^2 \theta_s \rangle = (1 + g^2)/2$ , and we recall that in unbounded RWs the distribution of  $\theta_n$  is a HG PF with  $g_n = g^n$ . The variance of  $s_{n+1} \cos \theta_n$  is therefore  $2\ell^2(1 + g^{2n})/2 - \ell^2 g^{2n} = \ell^2$ , irrespective of  $n$  and, for the 2D HG PF, of  $g$ . Consequently, variance  $(\langle z_N^2 \rangle - \langle z_N \rangle^2)/\ell^2 = N$ , irrespective of  $g$  for the 2D HG PF. The result is exact only for  $N = 0, 1, 2$ , i.e., before the 2<sup>nd</sup> scatter when cross-correlation terms arise in the counterpart of (A9) for  $z_N$ , and provides a lower bound at higher  $N$  in unbounded space.<sup>4</sup>

Most of the above analytical computations assumed a 2D HG PF and, accordingly, RWs in unbounded 2D space. Table A1 extends the investigation from 2D to 3D unbounded space, and to arbitrary PFs. None of the above conclusions are changed by these extensions.

Finally, we note that RWs in a half-space are more relevant to cloud image formation and can be easily investigated numerically. Figure A2a shows  $\langle z_N \rangle$  in that half-space scenario where the 2D RW still starts at  $z_0 = 0$  in the downward direction, normal to the  $z = 0$  plane ( $\theta_0 = 0$ ), but it is now terminated as soon as it crosses into the  $z < 0$  region. Thus, in contrast with the unbounded case, not all ( $10^6$ ) RWs populate all the orders-of-scattering, at least when  $n \geq 2$ . In fact, in the case of the 2D HG PF with  $g = 5/6$ , only  $\approx 1/3$  of the RWs are still alive at  $N = 100$ . We find that for the half-space RWs  $\langle z_N \rangle$  does not converge to a finite asymptote, for lack of negative values. Rather, it increases without bound. In contrast, confinement of the RW to  $z > 0$  reduces the standard deviation for  $z_N$  (Fig. A2b), but not for  $x_N$  (Fig. A2c).

TABLE A1. Recipes for HG and other PFs in unbounded 3D space. To compute  $\langle z_N \rangle/\ell$ , sum  $\langle \cos \theta_n \rangle$  in row #8 from 0 to  $N - 1$ . To compute a lower bound on  $(\langle z_N^2 \rangle - \langle z_N \rangle^2)/\ell^2$ , sum  $2\langle \cos^2 \theta_n \rangle - \langle \cos \theta_n \rangle^2$  in rows #8 and #9 from 0 to  $N - 1$ . To compute a lower bound on  $\langle x_N^2 \rangle/\ell^2$  ( $N \geq 1$ ), sum  $4\langle \sin^2 \theta_s \rangle \langle \cos^2 \theta_{n-1} \rangle$  in rows #7 and #9 from 1 to  $N - 1$ ; by convention,  $\langle x_0^2 \rangle = 0$ . Only constant-term and geometric series are involved. As an instance for the arbitrary 3D PF, the I3RC cloud droplet PSD used in the main text has  $h = 0.79$ .

| PF                                | 2D HG            | 3D HG                  | any 3D                        |
|-----------------------------------|------------------|------------------------|-------------------------------|
| expansion                         | Fourier cosine   | Legendre               | Legendre                      |
| coefficients                      | $a_i = g^i$      | $\eta_i = (2i + 1)g^i$ | arbitrary, after $\eta_0 = 1$ |
| ... for $\theta_n$                | $a_i^n$          | $(2i + 1)g^{ni}$       | $(2i + 1)^{1-n}\eta_i^n$      |
| $\langle \cos \theta_s \rangle$   | $g$              | $g$                    | $g = \eta_1/3$                |
| definition                        | $h = g^2$        | $h = g^2$              | $h = \eta_2/5$                |
| $\langle \cos^2 \theta_s \rangle$ | $(1 + g^2)/2$    | $(1 + 2g^2)/3$         | $(1 + 2h)/3$                  |
| $\langle \sin^2 \theta_s \rangle$ | $(1 - g^2)/2$    | $2(1 - g^2)/3$         | $2(1 - h)/3$                  |
| $\langle \cos \theta_n \rangle$   | $g^n$            | $g^n$                  | $g^n$                         |
| $\langle \cos^2 \theta_n \rangle$ | $(1 + g^{2n})/2$ | $(1 + 2g^{2n})/3$      | $(1 + 2h^n)/3$                |

We can now ask what is happening when multiply-scattered sunlight crosses the outer shell (OS) and reaches the veiled core (VC) from the standpoint of cloud tomography (Forster et al. 2021). In Fig. A2a, the VC boundary's optical depth of 5 is highlighted with a blue dot for the 2D half-space scenario, showing us that it corresponds to the mean penetration depth after  $\approx 6.5$  scatterings here, and  $\approx 7$  in 3D, with a more realistic PF for cloud droplets (not shown). At that point, Fig. A2b shows that the dispersion in penetration depth, as measured by the standard deviation  $(\langle z_N^2 \rangle - \langle z_N \rangle^2)^{1/2}$ , is  $\pm 2.5$  optical depths ( $\pm 2.7$  in 3D). Figure A2c then shows that the standard deviation  $\langle x_N^2 \rangle^{1/2} \approx 2.8$  ( $\approx 3.0$  in 3D), which is naturally comparable to  $(\langle z_N^2 \rangle - \langle z_N \rangle^2)^{1/2}$ . This in turn roughly defines the mean optical size of an “object” (e.g., a strong increase in local cloud opacity) that can be detected from the upper boundary or above, i.e., can impact significantly the cloud image by generating a detectable “feature.” Consequently, such a perturbation in cloud structure would likely not be detectable if embedded deeper (inside the the VC) rather than shallower (hence in the OS).

## References

- Davis, A., and A. Marshak, 1997: Lévy kinetics in slab geometry: Scaling of transmission probability. *Fractal Frontiers*, 63–72.
- Davis, A. B., 2002: Cloud remote sensing with sideways looks: Theory and first results using Multispectral Thermal Imager data. *Algorithms and Technologies for Multispectral, Hyperspectral, and Ultraspectral Imagery VIII*, International Society for Optics and Photonics, Vol. 4725, 397–405.
- Forster, L., A. B. Davis, D. J. Diner, and B. Mayer, 2021: Toward cloud tomography from space using misr and modis: Locating the “veiled core” in opaque convective clouds. *J. Atmos. Sci.*, **78**, 155–166.
- Henyey, L., and J. Greenstein, 1941: Diffuse radiation in the galaxy. *Astrophys. Journal*, **93**, 70–83.

<sup>4</sup> Also for  $N \geq 6$  in half-space RW domain, for this particular HG PF.

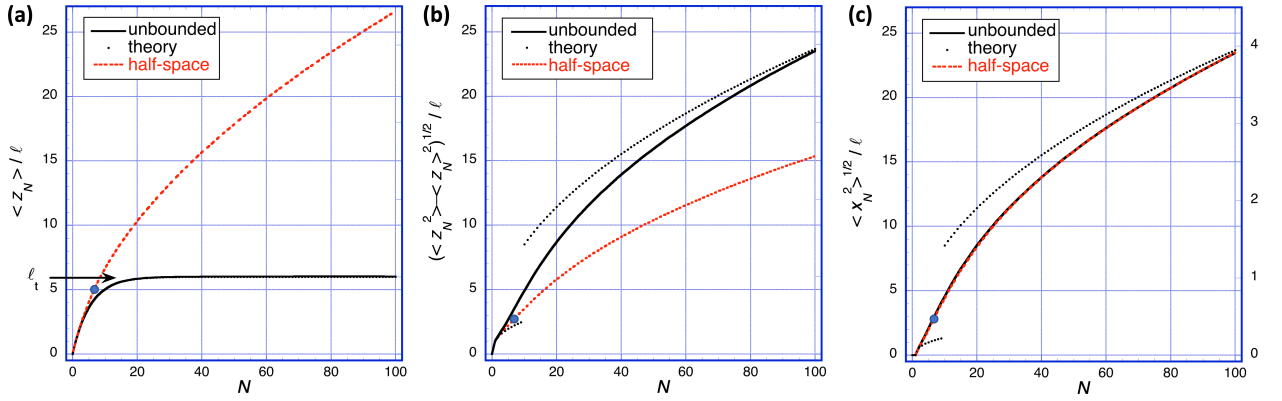

FIG. A2. Low-order statistics of 2D angularly-correlated RW coordinates (cf. Fig. A1) as functions of order-of-scattering  $N$  in unbounded space (solid, black) and a half-space (dashed, red), expressed in units of MFPs. Scale on the right is for the same quantities, but in units of transport MFPs. Steps are exponentially distributed with unit mean, and scattering angles were drawn from the 2D HG PF described in Fig. A1). (a) Mean of vertical coordinate  $z_N$  is plotted in units of MFP  $\ell$ , where we note that the theory in (A5) is exact and that  $\langle z_N \rangle$  asymptotes at the transport MFP  $\ell_t$ . By contrast, in the half-space scenario, the RW excursions into  $z < 0$  are terminated, so  $\langle z_N \rangle$  now increases without bound. (b) Standard deviation of vertical coordinate  $z_N$ , also in units of MFP  $\ell$ , is shown with theoretical predictions for the low and high ranges of  $N$ . In this case, the effect of terminating RWs at their first excursion into  $z < 0$  is to reduce significantly their dispersion in the  $z > 0$  space. (c) Same as (b), but for the horizontal coordinate  $x_N$ , again in units of MFP  $\ell$ . Here, the termination of RWs as soon as they land in  $z < 0$  territory makes no difference.
