# Supplementary material for: Toward Cloud Tomography from Space using MISR and MODIS: The Physics of Image Formation for Opaque Convective Clouds
Source: arXiv:2011.14537 ancillary file (2021-07-27)
Supplement: Supplementary file 2 [file paper_veiled_core_physics-eSupB.pdf]

## APPENDIX B

 **$R/T$  ratio for cylindrical clouds in the diffusion limit**

Davis (2002) showed that, for 3D spherical clouds, the  $R/T$  ratio equals  $(1 - g)\tau/2\chi$  in the radiative diffusion limit, and noted that the same is true for 1D plan-parallel slab clouds. Here,  $R$  is the fraction of incoming radiation that is reflected back to space, and  $T = 1 - R$  is the transmitted fraction in the absence of absorption (i.e., single scattering albedo  $\omega$  is unity). Furthermore,  $\tau$  is either the optical thickness of the slab cloud or the optical diameter of the spherical cloud. The asymmetry factor of the scattering phase function is denoted as usual by  $g$ , and  $\chi$  is an  $O(1)$  numerical factor discussed further and in the main text. Now, in the diffusion limit, radiative transfer (RT) is reduced to the solution of a Laplace or Helmholtz partial differential equation (PDE) on a segment in 1D space, and on a sphere in 3D space. Noting that, topologically, a segment is a ball in 1D space and a sphere is a ball in 3D space, we naturally ask about the circle, a ball in 2D space. Can we postulate that a cylindrical cloud (i.e., 2D diffusive RT in a circle) also has that  $R/T$  ratio?

A stronger motivation for exploring 2D RT is that in the previous study by Forster et al. (2021), we gained insights into 3D RT by using an idealized 2D cloud, asking ourselves

1. how far into a cloud can we “see” spatial structures in the cloud’s outer shell (OS) with realistic space-based imagers, and
2. how does the cloud’s veiled core (VC), where no detailed spatial structures can be seen, affect the cloud image.

The 1st question was addressed in Appendix A using angularly-correlated random walks (RWs) in 2D- or 3D-space and related RWs on the circle or sphere. In this Appendix, we simplify the 2nd task by considering a simple 2D cloud model that is entirely VC, hence where the RT is entirely in the diffusion regime.

In cylindrical coordinates, where  $\mathbf{x} = (\rho, \varphi, z)$ , the outer cloud boundary  $\partial C$  is defined as the surface where  $\rho = r$ . If the extinction coefficient in the cloud is  $\sigma_e$ , then its optical diameter is  $\tau = 2\sigma_e r$ . The distribution of incoming collimated solar irradiance across the cloud boundary is modeled as

$$F_{\text{in}}(\varphi) = F_0 \max\{\cos \varphi, 0\}, \quad (\text{B1})$$

with  $F_0$  denoting the solar constant and the anti-solar direction being  $\Omega_0 = (-1, 0, 0)$ .

Following Davis and Knyazikhin (2005), overall cloud reflection  $R$  is defined here as the ratio of  $\int_{F_{\text{in}}(\varphi) \geq 0} F_{\text{out}}(\varphi) r d\varphi$  to total cloud irradiance, namely,  $F_0 2r$ . Here,  $F_{\text{out}}(\varphi)$  is the outgoing flux at position  $(r, \varphi)$ ,

neglecting from now on the  $z$  coordinate since the problem is invariant under arbitrary translation in  $z$ .

In the diffusion limit, the radiance field is reduced to just two spherical harmonics in direction space:  $I(\mathbf{x}, \Omega) = [J(\mathbf{x}) + 3\Omega \cdot \mathbf{F}(\mathbf{x})]/4\pi$  in 3D space, where  $J(\mathbf{x})$  is scalar flux,  $\int_{4\pi} I(\mathbf{x}, \Omega) d\Omega$ , and  $\mathbf{F}(\mathbf{x})$  is vector flux,  $\int_{4\pi} \Omega I(\mathbf{x}, \Omega) d\Omega$ . The scattering phase function is also truncated at two spherical harmonics:  $p(\Omega \cdot \Omega') = [1 + 3g\Omega \cdot \Omega']/4\pi$ . Under these conditions, the 3D RT equation reduces to

- the exact expression of radiant energy conservation,  $\nabla \cdot \mathbf{F} = -\sigma_a J$ , in the absence of internal sources, with  $\sigma_a = (1 - \omega)\sigma_e$  being the absorption coefficient,
- and that of Fick’s approximate constitutive law,  $\mathbf{F} = -D\nabla J$ , where  $D$  is radiative diffusivity (in steady state). It can be shown that  $D = \ell_t/3$  where  $\ell_t = \ell/(1 - \omega g)$  is the transport or scaled MFP, with  $\ell = 1/\sigma_e$  being usual MFP.

In the absence of absorption ( $\sigma_a = 0$ , hence  $\omega = 1$ ), conservation and constitutive laws can be combined into  $\nabla^2 J = 0$ , where  $\nabla = (\partial_\rho, \rho^{-1}\partial_\varphi)$ .

In polar coordinates, where  $\mathbf{x} = (\rho, \varphi)$ , the solution of this 2D Laplace PDE that is both non-singular (finite at  $\rho = 0$ ) and symmetric in  $\varphi$  is expressed as

$$J(\rho, \varphi) = \sum_{m \geq 0} A_m \rho^m \cos m\varphi, \quad (\text{B2})$$

which reads as a Fourier cosine series. The unknown coefficients of this straightforward separation of variables are determined by matching the boundary condition (BC) that describes the  $\varphi$ -modulated solar illumination at the upper ( $|\varphi| \leq \pi/2$ ) semicircle, and no incoming irradiance from below; see Eq. (B1). In radiative diffusion theory, BCs are of the 3<sup>rd</sup> (a.k.a. Robin) type. In this case, we have

$$\frac{1}{4} \left( 1 + \chi \ell_t \frac{\partial}{\partial \rho} \right) J(\rho, \varphi) \Big|_{\rho=r} = F_{\text{in}}(\varphi), \quad (\text{B3})$$

where  $\chi \ell_t$  is the extrapolation length. In 3D space, the usual (so-called “Marshak”) choice for  $\chi$  is  $2/3$ , as rationalized in the main text (§3.a). In 2D space, the same argument based on the estimation of incoming flux  $F_{\text{in}}$ , knowing only scalar and vector fluxes ( $J, \|\mathbf{F}\|$ ) at the boundary, can be applied; it yields  $\chi = \pi/4$ .

Let  $f_m$  ( $m \geq 0$ ) be the Fourier coefficients in (B2), but for the incoming flux in (B1), where we can set  $F_0$  to unity without loss of generality. Thus, we have

$$f_m^{(\text{in})} = \frac{2 - \delta_{0,m}}{\pi} \int_0^\pi F_{\text{in}}(\varphi) \cos m\varphi d\varphi. \quad (\text{B4})$$

In view of the r.-h. side of (B1), we have  $f_0^{(\text{in})} = 1/\pi$ ,  $f_1^{(\text{in})} = 1/2$ ,  $f_m^{(\text{in})} = 2(-1)^{m/2+1}/(m^2 - 1)\pi$  for even  $m \geq 2$ ,

and  $f_m^{(\text{in})} = 0$  for odd  $m \geq 3$ . As for the l.-h. side of (B3), we find

$$F_{\text{in}}(\varphi) = \frac{1}{4} \sum_{m \geq 0} A_m r^m (1 + m\chi\ell_t/r) \cos m\varphi. \quad (\text{B5})$$

Term-by-term identification yields:  $A_0 = 4/\pi$ ,  $A_1 = 2/(1 + \chi\ell_t/r)r$ ,

$$A_m = \left(\frac{8}{\pi}\right) \frac{(-1)^{m/2+1}}{(m^2 - 1)(1 + m\chi\ell_t/r)r^m} \quad (\text{B6})$$

for even  $m \geq 2$ , and  $A_m = 0$  for odd  $m \geq 3$ .

By analogy with (B3) and (B5), the outgoing flux at  $\rho = r$  is

$$\begin{aligned} F_{\text{out}}(\varphi) &= \frac{1}{4} \left( 1 - \chi\ell_t \frac{\partial}{\partial \rho} \right) J(\rho, \varphi) \Big|_{\rho=r} \\ &= \frac{1}{4} \sum_{m \geq 0} A_m r^m (1 - m\chi\ell_t/r) \cos m\varphi. \end{aligned} \quad (\text{B7})$$

First, we can compute  $R + T = (1/4r) \int_0^\pi F_{\text{out}}(\varphi) r d\varphi$ , where only the 0<sup>th</sup>-order term survives:  $R + T = A_0 \times \pi/4$ , which is unity, as expected. Next, we compute  $R = (1/4r) \int_0^{\pi/2} F_{\text{out}}(\varphi) r d\varphi$ , where only the 0<sup>th</sup> and 1<sup>st</sup>-order terms survive:  $4R = A_0\pi/2 + A_1[1 - \chi\ell_t/r]r$ , while we also find that  $4T = A_0\pi/2 - A_1[1 - \chi\ell_t/r]r$ . A little algebra then leads to

$$\frac{R}{T} = \frac{r}{\chi\ell_t} = \frac{(1-g)\tau}{2\chi}. \quad (\text{B8})$$

As hypothesized, this is the same expression obtained by Davis (2002) for 3D spherical clouds as well as for 1D plan-parallel slab clouds. Figure B1 displays  $J(\rho, \varphi)$  from (B2) and the associated  $\mathbf{F}(\rho, \varphi)$  for two cases of 2D radiation diffusion through a circle. Setting  $\chi = \pi/4$  for 2D diffusion, the diffusion problem is solved for circles with  $r/\ell_t = 4/\pi$  (yielding  $R/T = 1$ ) and  $r/\ell_t = 40/\pi$  (yielding  $R/T = 10$ ). We note the steeper gradient in  $J$  cross the cloud for increased  $(1-g)\tau = 2r/\ell_t$  (top panel), and the enhanced curvature of the vector flux field (bottom panel). These lead to smaller  $T$ , and correspondingly larger  $R = 1 - T$ .

Numerical validation of the prediction in (B8) is presented in Fig. B2. A large number of 2D MC trajectories were launched from the upper semi-circular boundary of the cloud, either collimated in the anti-solar direction or in isotropically-distributed random directions. The latter option, in principle, mimics more closely the physics of diffusion theory, which is only expected to become valid for large optical diameters. Scattering is implemented with directional correlations according to the 2D version of the Henyey–Greenstein phase function (cf. Appendix A, Fig. A1) with  $g = 0.85$ . Optical diameter

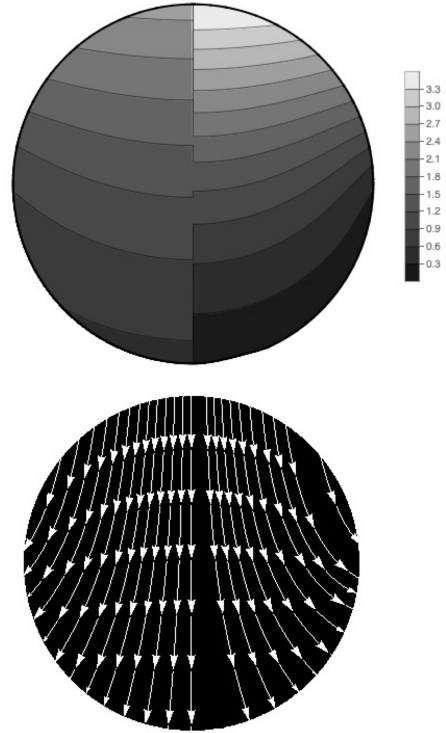

FIG. B1. 2D diffusive radiation transport across a circular medium, where we set  $\chi = \pi/4 \approx 0.7854$  in the Robin BCs expressed in (B3). Left-hand semi-circle is for  $2r/\ell_t = 8/\pi$  (scaled optical diameter  $\approx 2.55$ ), hence  $R/T = 1$  in (B8); right-hand counterpart is for a  $10\times$  smaller value of the transport MFP  $\ell_t$ , hence  $R/T = 10$ . Top:  $J(\rho, \varphi)$  fields on a common grayscale. Bottom: Streamlines for  $\mathbf{F}(\rho, \varphi) \propto -\nabla J$ .

$\tau = 2r/\ell$  was varied from 1 to 512 by successive divisions of  $\ell$  by factors of 2. In both collimated and isotropic illumination scenarios, the diffusion-theoretical prediction for  $R/T$  in (B8) is, as expected, accurate to within numerical accuracy, for the largest values of  $\tau$ . More specifically, the predicted dependence is approached as the *scaled* optical diameter  $\tau_t = (1-g)\tau$  reaches and exceeds unity.

## References

- Davis, A. B., 2002: Cloud remote sensing with sideways looks: Theory and first results using Multispectral Thermal Imager data. *Algorithms and Technologies for Multispectral, Hyperspectral, and Ultraspectral Imagery VIII*, International Society for Optics and Photonics, Vol. 4725, 397–405.
- Davis, A. B., and Y. Knyazikhin, 2005: A primer in 3D radiative transfer. *3D Radiative Transfer in Cloudy Atmospheres*, A. Marshak, and A. B. Davis, Eds., Springer, Heidelberg (Germany), chapter 3, 153–242.
- Forster, L., A. B. Davis, D. J. Diner, and B. Mayer, 2021: Toward cloud tomography from space using misr and modis: Locating the “veiled core” in opaque convective clouds. *Journal of the Atmospheric Sciences*, **78** (1), 155–166.

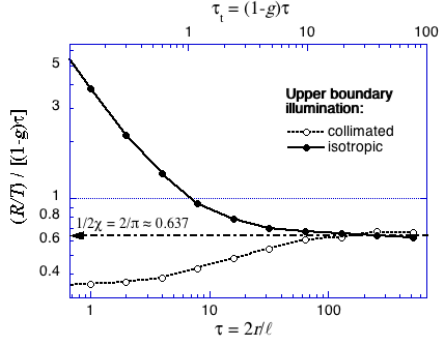

FIG. B2. 2D MC validation of  $R/T$  prediction in the asymptotic diffusion limit. Both collimated and isotropic illumination conditions were applied at the upper semi-circle boundary. The 2D Henyey-Greenstein phase function presented in Fig. A1 was used, with asymmetry factor  $g = 0.85$ . The optical diameter  $\tau = 2r/\ell$  of the circle was varied by factors of 2, from 1 to 512, along the lower horizontal axis. The upper horizontal axis is scaled optical diameter  $\tau_t = (1 - g)\tau$ . Vertically, we plot  $(R/T)/\tau_t$ , which is predicted in (B8) to be  $1/2\chi = 2/\pi \approx 0.637$  in 2D. This prediction becomes increasingly accurate as  $\tau_t$  increases beyond unity.

©2021 California Institute of Technology. Government sponsorship acknowledged.
